# Supplementary material for: MSCEqF: A Multi State Constraint Equivariant Filter for Vision-aided Inertial Navigation
Source: arXiv:2311.11649 source file (2023-11-20)
Supplement: Supplementary file 1 [file appendix.tex]

\subsection{Algorithm}
The proposed \ac{msceqf} is implemented as a C++ stand-alone library. The main modules are here described.

\subsubsection{Vision frontend}
Once an image is recorded, and the number of tracked features goes below a given threshold, new visual features are detected. The \ac{msceqf} vision frontend is built upon~\cite{opencv_library}, and performs multi-threaded feature detection on the image divided in cells and in multiple pyramids via a multi-choice feature detector, FAST~\cite{rosten2006machine} or Shi-Tomasi~\cite{shi1994good}. Detected features are then tracked temporally with KLT optical flow~\cite{lucas1981iterative, tomasi1991detection}, and stored in tracks to be used for filter updates.

% \subsubsection{Filter origin initialization}
% The \ac{msceqf} state $\hat{X}$ is initialized at identity. However, the origin state $\xizero$ is initialized with an estimate of the initial conditions. Such initialization is done assuming static condition at the beginning, and hence computing the roll and pitch angles within $\mathring{\Rot{}{}}$, together with the \ac{imu} biases $\mathring{\Vector{}{b}{}}$, from the \ac{imu} measurements collected during the static phase, by assuming the \ac{imu} measures zero angular velocity and the gravity vector. To distinguish between static and motion phases we employ a check based on both the \ac{imu} readings and the image disparity.

\subsubsection{Filter main loop}
The main loop of the \ac{msceqf} present significant similarities to that of the original \ac{msckf} formulation~\cite{Mourikis2007ANavigation}, albeit with a few distinctions.
Firstly, the presented \ac{msceqf} supports online camera extrinsics and intrinsics calibration. Furthermore, during the propagation phase of the filter, \equref{lifted_vins} is integrated with a Lie group integrator employing the exponential map of the symmetry group. Additionally, the \ac{msceqf} update supports multiple feature parameterization including \emph{anchored euclidean}, \emph{anchored inverse depth}, and \emph{anchored polar}, which is the anchored version of the recently presented polar parametrization~\cite{vanGoor2022EqVIO:Odometry}.
